# Supplementary material for: Integrated Study of NGC 1662, NGC 1778, NGC 2422, and NGC 2437 Open Clusters: from Stellar Parameters to Orbital Trajectories Utilizing Gaia DR3 Archive
Source: arXiv:2611.29413 source file (2026-11-22)
Supplement: Supplementary file 1 [file Supplementary_File_Electronic_Table.tex]

\begin{table*} \footnotesize
\centering
\caption{Radial velocity measurements for NGC 1662}
\begin{tabular}{l c c c c c c c c l}
%\begin{tabularx}{\linewidth}{l c c c c c c c c l}
\hline\hline
ID & $\alpha$ (hh:mm:ss) & $\delta$ (dd:mm:ss) & $G$ (mag) & $P$ & $V_R$ (km s$^{-1}$)& $\sigma_{V_R}$ & & RUWE & Survey \\
\hline
1 & 04:46:38.00 & +10:39:53.9 & 14.81 & 0.96 & -1.07 & 6.78 & & 1.02 & Gaia DR3 \\
2 & 04:46:42.44 & +11:08:50.5 & 11.81 & 1.00 & -12.67 & 1.90 & & 1.14 & LAMOST \\
3 & 04:46:47.24 & +10:37:55.2 & 12.71 & 1.00 & -13.11 & 2.08 & & 1.00 & LAMOST \\
4 & 04:46:50.04 & +11:10:47.6 & 13.74 & 0.97 & -19.47 & 4.41 & & 1.14 & Gaia DR3 \\
5 & 04:46:51.19 & +11:19:54.0 & 11.64 & 1.00 & -7.68 & 5.29 & & 1.19 & LAMOST \\
6 & 04:47:04.93 & +11:22:59.0 & 14.56 & 1.00 & -7.18 & 4.96 & & 0.98 & LAMOST \\
7 & 04:47:16.87 & +10:43:26.1 & 10.12 & 0.98 & -21.73 & 3.22 & & 1.16 & Gaia DR3 \\
8 & 04:47:29.10 & +10:50:44.9 & 14.30 & 1.00 & -9.85 & 4.01 & & 1.38 & LAMOST \\
9 & 04:47:30.71 & +11:44:18.5 & 13.23 & 1.00 & -11.47 & 2.18 & & 1.07 & LAMOST \\
10 & 04:47:43.17 & +10:40:51.8 & 14.69 & 0.98 & -21.34 & 8.11 & & 0.97 & Gaia DR3 \\
11 & 04:47:43.56 & +10:39:05.2 & 14.08 & 1.00 & -15.56 & 2.98 & & 1.01 & LAMOST \\
12 & 04:47:46.85 & +10:20:03.3 & 9.35 & 0.95 & -17.75 & 1.86 & & 0.94 & Gaia DR3 \\
13 & 04:47:47.13 & +10:52:39.6 & 13.94 & 0.98 & -12.18 & 2.75 & & 1.02 & Gaia DR3 \\
14 & 04:47:48.31 & +10:38:32.7 & 13.72 & 0.98 & -13.92 & 2.55 & & 1.00 & Gaia DR3 \\
15 & 04:47:49.62 & +11:04:25.3 & 13.95 & 1.00 & -10.27 & 2.76 & & 1.15 & LAMOST \\
16 & 04:47:52.01 & +10:47:05.2 & 13.96 & 1.00 & -10.46 & 3.88 & & 1.04 & LAMOST \\
17 & 04:47:53.04 & +10:52:58.4 & 11.35 & 1.00 & -21.72 & 4.67 & & 1.14 & Gaia DR3 \\
18 & 04:47:53.33 & +10:52:34.3 & 15.08 & 1.00 & -16.94 & 5.24 & & 1.04 & LAMOST \\
19 & 04:47:55.68 & +11:52:53.0 & 13.28 & 1.00 & -12.59 & 2.34 & & 1.06 & LAMOST \\
20 & 04:48:00.57 & +10:57:10.7 & 10.06 & 0.99 & -13.55 & 1.14 & & 0.99 & Gaia DR3 \\
21 & 04:48:04.94 & +10:59:21.2 & 11.59 & 1.00 & -13.13 & 0.83 & & 1.01 & Gaia DR3 \\
22 & 04:48:09.46 & +10:51:52.0 & 14.54 & 0.99 & -11.98 & 4.40 & & 1.03 & Gaia DR3 \\
23 & 04:48:09.87 & +11:35:44.2 & 14.31 & 1.00 & -14.39 & 3.07 & & 1.10 & LAMOST \\
24 & 04:48:10.86 & +11:40:12.5 & 11.63 & 1.00 & -11.85 & 3.08 & & 1.10 & LAMOST \\
25 & 04:48:15.12 & +11:00:33.8 & 11.22 & 0.99 & -15.78 & 1.37 & & 1.13 & Gaia DR3 \\
26 & 04:48:25.18 & +10:47:05.8 & 10.67 & 0.99 & -19.08 & 1.60 & & 1.02 & Gaia DR3 \\
27 & 04:48:25.49 & +10:36:36.8 & 14.26 & 0.98 & -13.40 & 4.30 & & 1.11 & Gaia DR3 \\
28 & 04:48:27.36 & +10:49:48.3 & 10.98 & 1.00 & -13.27 & 1.65 & & 1.05 & LAMOST \\
29 & 04:48:27.51 & +11:13:33.9 & 13.78 & 1.00 & 8.59 & 3.67 & & 1.02 & LAMOST \\
30 & 04:48:27.87 & +10:55:45.7 & 10.24 & 0.98 & -25.95 & 3.40 & & 1.02 & Gaia DR3 \\
31 & 04:48:29.51 & +10:55:48.3 & 7.95 & 1.00 & -13.76 & 0.12 & & 0.95 & Gaia DR3 \\
32 & 04:48:32.08 & +10:57:59.0 & 8.42 & 1.00 & -12.90 & 0.12 & & 0.94 & Gaia DR3 \\
33 & 04:48:32.13 & +11:35:51.9 & 11.87 & 1.00 & -12.61 & 3.33 & & 1.19 & Gaia DR3 \\
34 & 04:48:33.82 & +10:55:52.8 & 14.51 & 0.97 & -13.11 & 3.66 & & 1.04 & Gaia DR3 \\
35 & 04:48:35.45 & +11:00:17.0 & 13.36 & 0.99 & -13.18 & 1.83 & & 1.03 & Gaia DR3 \\
36 & 04:48:37.75 & +11:23:23.2 & 14.83 & 0.97 & -8.67 & 4.51 & & 1.09 & Gaia DR3 \\
37 & 04:48:41.96 & +10:53:54.1 & 13.09 & 1.00 & -9.72 & 1.65 & & 1.01 & LAMOST \\
38 & 04:48:42.21 & +10:59:33.3 & 10.60 & 0.99 & -19.14 & 2.62 & & 0.93 & Gaia DR3 \\
39 & 04:48:42.94 & +10:25:20.4 & 14.90 & 0.98 & -20.75 & 5.40 & & 1.01 & Gaia DR3 \\
40 & 04:48:43.30 & +10:50:32.0 & 12.07 & 1.00 & -9.73 & 1.40 & & 1.06 & LAMOST \\
41 & 04:48:43.43 & +11:33:04.0 & 12.38 & 1.00 & -9.48 & 2.42 & & 0.95 & Gaia DR3 \\
42 & 04:48:49.01 & +10:29:36.7 & 14.74 & 0.98 & -15.41 & 7.02 & & 0.99 & Gaia DR3 \\
43 & 04:48:50.04 & +10:57:34.1 & 14.05 & 1.00 & -12.29 & 2.47 & & 1.06 & LAMOST \\
44 & 04:48:51.15 & +10:32:08.8 & 15.33 & 0.97 & -3.71 & 5.86 & & 1.10 & Gaia DR3 \\
45 & 04:48:53.68 & +10:42:42.2 & 11.65 & 1.00 & -12.79 & 0.50 & & 1.28 & LAMOST \\
46 & 04:48:55.92 & +11:12:50.9 & 12.79 & 1.00 & -12.26 & 2.60 & & 1.00 & Gaia DR3 \\
47 & 04:48:58.17 & +10:54:33.3 & 13.76 & 1.00 & -11.94 & 1.95 & & 0.99 & LAMOST \\
48 & 04:48:59.71 & +11:48:17.2 & 13.39 & 1.00 & -12.91 & 2.73 & & 0.98 & LAMOST \\
49 & 04:49:01.21 & +11:41:57.2 & 14.70 & 0.95 & -13.31 & 4.48 & & 1.08 & Gaia DR3 \\
50 & 04:49:02.62 & +10:14:32.4 & 12.18 & 1.00 & -3.93 & 4.00 & & 0.98 & Gaia DR3 \\
51 & 04:49:03.20 & +11:01:51.0 & 13.96 & 1.00 & -11.42 & 2.54 & & 1.01 & LAMOST \\
52 & 04:49:04.61 & +11:40:09.7 & 11.10 & 0.97 & -20.73 & 3.47 & & 1.17 & Gaia DR3 \\
53 & 04:49:06.82 & +10:40:27.9 & 13.73 & 1.00 & -14.59 & 2.99 & & 1.39 & LAMOST \\
54 & 04:49:07.18 & +10:42:48.1 & 12.37 & 1.00 & -13.75 & 3.44 & & 1.30 & Gaia DR3 \\
55 & 04:49:07.69 & +10:15:53.6 & 14.70 & 0.92 & -3.03 & 9.10 & & 0.99 & Gaia DR3 \\
56 & 04:49:10.71 & +10:44:52.4 & 12.73 & 1.00 & -10.71 & 2.20 & & 1.11 & LAMOST \\
57 & 04:49:17.88 & +10:39:53.0 & 10.59 & 0.99 & -20.01 & 2.20 & & 1.06 & Gaia DR3 \\
58 & 04:49:20.51 & +11:17:24.5 & 12.27 & 1.00 & -14.90 & 1.70 & & 1.08 & LAMOST \\
59 & 04:49:24.94 & +11:23:47.5 & 12.88 & 1.00 & -10.48 & 1.17 & & 0.93 & LAMOST \\
60 & 04:49:25.99 & +10:51:41.1 & 10.65 & 0.99 & -16.40 & 2.82 & & 1.00 & Gaia DR3 \\
61 & 04:49:26.27 & +10:41:12.6 & 11.47 & 1.00 & -9.73 & 1.91 & & 1.28 & Gaia DR3 \\
62 & 04:49:27.57 & +10:38:56.8 & 13.75 & 0.99 & -14.26 & 3.71 & & 0.99 & Gaia DR3 \\
63 & 04:49:28.46 & +10:40:19.2 & 11.69 & 0.99 & -15.53 & 2.86 & & 1.30 & Gaia DR3 \\
64 & 04:49:31.03 & +10:44:13.8 & 12.34 & 1.00 & -14.99 & 1.67 & & 1.10 & LAMOST \\
65 & 04:49:33.12 & +11:27:23.6 & 14.41 & 1.00 & -6.29 & 1.92 & & 0.97 & LAMOST \\
66 & 04:49:38.31 & +10:42:22.4 & 11.79 & 0.99 & -11.19 & 1.74 & & 1.12 & Gaia DR3 \\
67 & 04:49:39.59 & +10:37:41.5 & 14.00 & 0.98 & -13.64 & 3.43 & & 1.01 & Gaia DR3 \\
68 & 04:49:48.72 & +10:45:28.7 & 10.07 & 0.99 & -17.21 & 2.11 & & 1.07 & Gaia DR3 \\
69 & 04:50:16.99 & +11:50:43.9 & 13.93 & 1.00 & -12.63 & 2.82 & & 1.32 & LAMOST \\
70 & 04:50:31.50 & +10:58:52.5 & 9.54 & 0.98 & -18.75 & 1.49 & & 0.98 & Gaia DR3 \\
71 & 04:50:43.24 & +10:13:57.1 & 14.28 & 0.91 & -10.33 & 3.86 & & 1.01 & Gaia DR3 \\
72 & 04:50:43.77 & +10:44:36.7 & 12.79 & 1.00 & -12.00 & 2.73 & & 1.05 & Gaia DR3 \\
73 & 04:50:45.36 & +11:06:24.1 & 13.50 & 0.98 & -11.85 & 2.52 & & 1.04 & Gaia DR3 \\
74 & 04:50:50.39 & +10:59:09.8 & 14.30 & 0.98 & -14.62 & 3.83 & & 1.06 & Gaia DR3 \\
75 & 04:50:55.70 & +10:44:59.7 & 13.85 & 1.00 & -12.41 & 2.64 & & 1.07 & LAMOST \\
76 & 04:50:56.59 & +10:31:05.8 & 14.23 & 0.96 & -10.32 & 2.54 & & 1.03 & Gaia DR3 \\
77 & 04:51:18.71 & +11:52:38.0 & 14.46 & 0.62 & -11.80 & 5.79 & & 0.99 & Gaia DR3 \\
78 & 04:51:20.55 & +11:04:04.6 & 14.65 & 0.97 & -8.35 & 3.76 & & 1.02 & Gaia DR3 \\
\hline
\end{tabular}
\label{tab:NGC_1662}
\end{table*}

% Tablo: NGC_1778
\begin{table*} \footnotesize
\centering
\caption{Radial velocity measurements for NGC 1778}
\begin{tabular}{l c c c c c c c c l}
\hline\hline
ID & $\alpha$ (hh:mm:ss) & $\delta$ (dd:mm:ss) & $G$ (mag) & $P$ & $V_R$ (km s$^{-1}$)& $\sigma_{V_R}$ & & RUWE & Survey \\
\hline
1 & 05:07:00.89 & +37:04:34.3 & 14.33 & 0.97 & -14.41 & 2.09 & & 1.03 & Gaia DR3 \\
2 & 05:07:02.46 & +36:55:26.5 & 14.74 & 0.92 & -15.06 & 2.58 & & 1.03 & Gaia DR3 \\
3 & 05:07:48.17 & +37:13:50.3 & 11.85 & 0.99 & -16.85 & 18.42 & & 1.35 & Gaia DR3 \\
4 & 05:07:55.72 & +37:19:57.9 & 11.97 & 1.00 & 42.25 & 0.22 & & 1.12 & Gaia DR3 \\
5 & 05:07:59.79 & +37:02:12.3 & 11.61 & 1.00 & 24.61 & 16.90 & & 1.29 & Gaia DR3 \\
6 & 05:08:01.30 & +36:59:18.0 & 11.64 & 1.00 & 6.44 & 9.51 & & 1.25 & Gaia DR3 \\
7 & 05:08:03.50 & +37:10:33.2 & 14.78 & 0.99 & 0.59 & 7.83 & & 1.04 & Gaia DR3 \\
8 & 05:08:03.88 & +36:57:36.7 & 9.43 & 0.99 & 4.89 & 0.63 & & 1.35 & Gaia DR3 \\
9 & 05:08:15.54 & +37:02:47.3 & 14.44 & 1.00 & 7.21 & 21.87 & & 1.02 & Gaia DR3 \\
10 & 05:08:20.29 & +37:06:24.3 & 10.77 & 1.00 & -26.11 & 0.19 & & 0.92 & Gaia DR3 \\
11 & 05:08:21.75 & +37:06:42.4 & 11.54 & 1.00 & -6.21 & 24.85 & & 1.40 & Gaia DR3 \\
12 & 05:08:43.35 & +36:54:20.9 & 12.36 & 0.99 & 20.39 & 25.90 & & 0.94 & Gaia DR3 \\
13 & 05:08:49.56 & +37:01:25.9 & 12.22 & 1.00 & 11.10 & 22.20 & & 1.06 & Gaia DR3 \\
14 & 05:09:34.89 & +36:52:19.0 & 12.87 & 1.00 & -77.09 & 0.44 & & 0.97 & LAMOST \\
15 & 05:09:37.66 & +36:54:46.5 & 14.18 & 1.00 & -63.22 & 1.44 & & 1.11 & LAMOST \\
16 & 05:09:58.65 & +36:39:45.9 & 14.60 & 1.00 & -39.35 & 2.55 & & 1.08 & LAMOST \\
\hline
\end{tabular}
\label{tab:NGC_1778}
\end{table*}

% Tablo: NGC_2422
\begin{table*} \footnotesize
\centering
\caption{Radial velocity measurements for NGC 2422}
\begin{tabular}{l c c c c c c c c l}
\hline\hline
ID & $\alpha$ (hh:mm:ss) & $\delta$ (dd:mm:ss) & $G$ (mag) & $P$ & $V_R$ (km s$^{-1}$)& $\sigma_{V_R}$ & & RUWE & Survey \\
\hline
1 & 07:32:11.90 & -14:08:20.8 & 14.84 & 0.80 & -43.28 & 8.04 & & 0.95 & Gaia DR3 \\
2 & 07:32:52.49 & -13:41:58.4 & 10.57 & 0.80 & 28.17 & 3.16 & & 0.91 & Gaia DR3 \\
3 & 07:32:56.34 & -14:50:24.9 & 10.59 & 0.97 & 24.80 & 4.06 & & 1.03 & Gaia DR3 \\
4 & 07:33:07.88 & -15:10:42.2 & 9.26 & 0.54 & 42.93 & 5.68 & & 1.00 & Gaia DR3 \\
5 & 07:33:16.99 & -14:22:59.6 & 12.01 & 1.00 & 50.10 & 1.00 & & 0.93 & Gaia DR3 \\
6 & 07:33:26.43 & -13:48:38.2 & 10.57 & 0.93 & 33.11 & 1.95 & & 0.89 & Gaia DR3 \\
7 & 07:33:38.68 & -14:33:18.4 & 14.00 & 0.95 & 35.00 & 3.87 & & 1.02 & Gaia DR3 \\
8 & 07:33:47.23 & -15:20:14.2 & 14.71 & 0.53 & 29.22 & 6.15 & & 0.96 & Gaia DR3 \\
9 & 07:33:52.33 & -13:50:20.8 & 12.38 & 1.00 & 36.97 & 2.42 & & 0.92 & Gaia DR3 \\
10 & 07:33:56.28 & -15:03:42.9 & 10.88 & 0.64 & 33.77 & 4.14 & & 1.04 & Gaia DR3 \\
11 & 07:34:07.17 & -14:34:42.1 & 11.74 & 0.99 & 33.59 & 1.11 & & 1.27 & Gaia DR3 \\
12 & 07:34:10.58 & -14:42:57.4 & 13.86 & 0.99 & 34.51 & 3.46 & & 1.02 & Gaia DR3 \\
13 & 07:34:19.60 & -14:14:19.7 & 14.96 & 0.99 & 14.62 & 15.13 & & 0.99 & Gaia DR3 \\
14 & 07:34:22.27 & -14:08:41.6 & 12.29 & 1.00 & 35.83 & 3.44 & & 0.92 & Gaia DR3 \\
15 & 07:34:22.30 & -13:51:55.9 & 14.43 & 0.98 & 34.17 & 4.91 & & 1.01 & Gaia DR3 \\
16 & 07:34:39.77 & -13:58:11.2 & 14.43 & 0.95 & 30.13 & 3.89 & & 1.01 & Gaia DR3 \\
17 & 07:34:41.90 & -13:59:14.5 & 12.09 & 1.00 & 18.07 & 6.14 & & 1.28 & Gaia DR3 \\
18 & 07:34:45.40 & -15:06:33.4 & 14.67 & 0.98 & 36.71 & 4.52 & & 1.09 & Gaia DR3 \\
19 & 07:34:45.51 & -14:19:18.6 & 12.66 & 0.94 & -2.43 & 35.40 & & 0.93 & Gaia DR3 \\
20 & 07:34:47.41 & -13:58:33.5 & 10.26 & 0.98 & 33.24 & 0.85 & & 1.01 & Gaia DR3 \\
21 & 07:34:56.28 & -14:21:56.2 & 11.71 & 1.00 & 35.77 & 1.16 & & 0.87 & Gaia DR3 \\
22 & 07:35:02.96 & -15:34:34.6 & 13.17 & 0.82 & 32.24 & 3.36 & & 0.90 & Gaia DR3 \\
23 & 07:35:05.08 & -14:34:27.5 & 14.57 & 1.00 & 38.77 & 4.63 & & 1.12 & Gaia DR3 \\
24 & 07:35:05.31 & -14:02:41.1 & 9.89 & 0.99 & 32.61 & 0.77 & & 0.93 & Gaia DR3 \\
25 & 07:35:13.02 & -14:48:11.3 & 12.53 & 1.00 & 34.10 & 5.01 & & 0.97 & Gaia DR3 \\
26 & 07:35:16.22 & -14:42:53.6 & 10.92 & 1.00 & 40.11 & 2.04 & & 0.89 & RAVE \\
27 & 07:35:17.58 & -15:05:46.6 & 14.51 & 0.99 & 28.36 & 5.47 & & 1.03 & Gaia DR3 \\
28 & 07:35:18.10 & -14:48:31.0 & 14.14 & 1.00 & 36.16 & 3.52 & & 0.99 & Gaia DR3 \\
29 & 07:35:18.84 & -14:39:44.3 & 14.30 & 1.00 & 39.93 & 4.28 & & 1.00 & Gaia DR3 \\
30 & 07:35:19.53 & -14:07:17.7 & 11.33 & 1.00 & 36.10 & 1.20 & & 1.05 & Gaia DR3 \\
31 & 07:35:19.61 & -14:59:14.5 & 13.22 & 0.99 & 37.27 & 2.86 & & 0.95 & Gaia DR3 \\
32 & 07:35:22.38 & -13:18:00.2 & 12.79 & 1.00 & 36.99 & 3.19 & & 0.95 & Gaia DR3 \\
33 & 07:35:23.88 & -14:46:52.6 & 14.65 & 0.99 & 39.05 & 4.70 & & 0.98 & Gaia DR3 \\
34 & 07:35:28.44 & -15:37:30.2 & 14.28 & 0.73 & 42.74 & 3.70 & & 1.02 & Gaia DR3 \\
35 & 07:35:30.91 & -14:29:22.0 & 12.16 & 1.00 & 31.83 & 2.45 & & 0.89 & Gaia DR3 \\
36 & 07:35:31.48 & -14:36:22.6 & 14.91 & 0.99 & 44.62 & 6.76 & & 1.01 & Gaia DR3 \\
37 & 07:35:31.54 & -13:33:19.3 & 13.33 & 0.96 & 36.21 & 2.93 & & 0.96 & Gaia DR3 \\
38 & 07:35:31.67 & -14:27:10.6 & 10.08 & 1.00 & 30.17 & 6.31 & & 0.83 & Gaia DR3 \\
39 & 07:35:32.26 & -14:34:01.8 & 11.29 & 1.00 & 35.24 & 1.79 & & 1.04 & Gaia DR3 \\
40 & 07:35:33.54 & -14:22:11.7 & 14.36 & 1.00 & 34.79 & 3.95 & & 1.06 & Gaia DR3 \\
41 & 07:35:36.28 & -14:40:13.9 & 8.80 & 1.00 & 37.27 & 1.86 & & 1.08 & Gaia DR3 \\
42 & 07:35:39.10 & -14:02:33.1 & 11.39 & 1.00 & 39.60 & 2.04 & & 1.02 & RAVE \\
43 & 07:35:39.17 & -14:29:48.6 & 14.43 & 1.00 & 37.47 & 5.75 & & 0.91 & Gaia DR3 \\
44 & 07:35:41.48 & -14:37:30.2 & 14.78 & 1.00 & 35.66 & 6.04 & & 0.96 & Gaia DR3 \\
45 & 07:35:44.00 & -13:18:00.0 & 11.96 & 1.00 & 39.00 & 10.82 & & 0.89 & Gaia DR3 \\
46 & 07:35:47.11 & -14:10:28.0 & 11.26 & 1.00 & 44.06 & 4.45 & & 0.98 & Gaia DR3 \\
47 & 07:35:47.28 & -14:30:41.2 & 13.07 & 1.00 & 33.87 & 3.17 & & 1.05 & Gaia DR3 \\
48 & 07:35:47.39 & -14:19:00.0 & 14.84 & 1.00 & 40.34 & 4.55 & & 1.02 & Gaia DR3 \\
49 & 07:35:49.28 & -14:22:26.1 & 13.27 & 0.99 & 31.72 & 4.34 & & 1.10 & Gaia DR3 \\
50 & 07:35:49.59 & -14:57:00.8 & 14.89 & 0.97 & 43.00 & 3.99 & & 0.94 & Gaia DR3 \\
51 & 07:35:50.30 & -15:10:52.1 & 12.44 & 1.00 & 21.30 & 4.20 & & 0.84 & Gaia DR3 \\
52 & 07:35:50.57 & -14:57:53.0 & 12.11 & 1.00 & 37.51 & 2.76 & & 0.91 & Gaia DR3 \\
53 & 07:35:50.77 & -14:37:49.5 & 12.82 & 1.00 & 33.31 & 1.20 & & 1.05 & Gaia DR3 \\
54 & 07:35:50.85 & -14:11:18.3 & 12.54 & 1.00 & 41.46 & 4.63 & & 0.93 & Gaia DR3 \\
55 & 07:35:53.15 & -14:26:41.5 & 11.57 & 1.00 & 37.48 & 1.34 & & 0.91 & Gaia DR3 \\
56 & 07:35:53.22 & -14:35:30.3 & 10.71 & 1.00 & 12.29 & 9.95 & & 1.16 & Gaia DR3 \\
57 & 07:35:54.38 & -14:21:09.1 & 13.59 & 1.00 & 32.84 & 3.07 & & 1.01 & Gaia DR3 \\
58 & 07:35:54.67 & -14:44:37.4 & 13.10 & 1.00 & 33.00 & 2.38 & & 1.04 & Gaia DR3 \\
59 & 07:35:54.95 & -14:52:34.6 & 14.71 & 1.00 & 29.94 & 5.08 & & 1.02 & Gaia DR3 \\
60 & 07:35:56.96 & -14:42:39.0 & 7.93 & 1.00 & 44.46 & 1.08 & & 0.93 & Gaia DR3 \\
61 & 07:35:57.52 & -14:32:40.7 & 12.26 & 1.00 & -8.83 & 10.31 & & 1.11 & Gaia DR3 \\
62 & 07:35:57.69 & -14:16:26.2 & 11.04 & 1.00 & 35.94 & 3.00 & & 1.31 & Gaia DR3 \\
63 & 07:35:58.20 & -14:14:24.0 & 13.50 & 1.00 & 33.41 & 3.35 & & 1.35 & Gaia DR3 \\
64 & 07:35:59.77 & -15:00:05.7 & 13.82 & 1.00 & 23.67 & 5.66 & & 0.97 & Gaia DR3 \\
65 & 07:36:01.64 & -14:19:23.0 & 14.53 & 1.00 & 34.50 & 4.98 & & 1.04 & Gaia DR3 \\
66 & 07:36:04.70 & -14:29:18.1 & 9.78 & 1.00 & 22.44 & 6.50 & & 0.82 & Gaia DR3 \\
67 & 07:36:05.38 & -14:38:22.9 & 13.29 & 1.00 & 32.33 & 4.21 & & 1.15 & Gaia DR3 \\
68 & 07:36:08.08 & -14:29:42.1 & 12.57 & 1.00 & 33.88 & 2.58 & & 1.30 & Gaia DR3 \\
69 & 07:36:08.88 & -14:30:36.8 & 12.25 & 1.00 & 37.72 & 2.22 & & 0.91 & Gaia DR3 \\
70 & 07:36:09.88 & -14:40:17.4 & 10.49 & 1.00 & 33.69 & 4.73 & & 0.97 & Gaia DR3 \\
71 & 07:36:10.70 & -14:50:44.0 & 14.39 & 1.00 & 40.52 & 5.49 & & 1.08 & Gaia DR3 \\
72 & 07:36:10.71 & -14:27:40.9 & 9.88 & 1.00 & 30.13 & 4.09 & & 0.91 & Gaia DR3 \\
73 & 07:36:10.78 & -14:22:48.8 & 9.96 & 1.00 & 31.84 & 3.84 & & 0.84 & Gaia DR3 \\
74 & 07:36:10.98 & -15:04:45.6 & 14.57 & 0.99 & 61.92 & 10.58 & & 1.04 & Gaia DR3 \\
75 & 07:36:11.76 & -14:37:16.9 & 13.57 & 1.00 & 38.87 & 2.84 & & 1.11 & Gaia DR3 \\
76 & 07:36:12.17 & -14:38:02.4 & 10.96 & 1.00 & 36.42 & 2.45 & & 1.17 & RAVE \\
77 & 07:36:12.17 & -14:26:38.5 & 13.65 & 1.00 & 37.27 & 4.04 & & 1.03 & Gaia DR3 \\
78 & 07:36:12.98 & -14:52:18.6 & 14.21 & 1.00 & 35.92 & 3.48 & & 1.02 & Gaia DR3 \\
79 & 07:36:14.18 & -14:23:46.7 & 11.97 & 1.00 & 30.42 & 2.73 & & 1.24 & Gaia DR3 \\
80 & 07:36:14.37 & -14:40:27.6 & 12.87 & 1.00 & 32.27 & 2.82 & & 1.13 & Gaia DR3 \\
81 & 07:36:14.61 & -14:34:11.3 & 10.70 & 1.00 & 34.10 & 2.28 & & 1.05 & Gaia DR3 \\
82 & 07:36:14.64 & -14:20:49.4 & 13.80 & 1.00 & 37.81 & 3.42 & & 0.97 & Gaia DR3 \\
83 & 07:36:15.22 & -14:35:43.2 & 11.63 & 1.00 & 37.91 & 0.98 & & 0.91 & Gaia DR3 \\
84 & 07:36:15.53 & -14:22:22.5 & 13.66 & 1.00 & 30.97 & 4.00 & & 1.04 & Gaia DR3 \\
85 & 07:36:17.88 & -13:48:37.1 & 14.58 & 0.99 & 33.92 & 4.82 & & 1.07 & Gaia DR3 \\
86 & 07:36:17.93 & -14:55:40.6 & 13.10 & 1.00 & 35.74 & 5.59 & & 1.04 & Gaia DR3 \\
87 & 07:36:17.96 & -13:19:13.9 & 9.76 & 0.60 & 24.08 & 3.27 & & 1.00 & Gaia DR3 \\
88 & 07:36:18.18 & -14:15:42.6 & 14.77 & 1.00 & 37.99 & 11.73 & & 1.08 & Gaia DR3 \\
89 & 07:36:18.60 & -14:22:59.8 & 12.96 & 1.00 & 31.65 & 2.56 & & 1.02 & Gaia DR3 \\
90 & 07:36:20.26 & -14:20:24.2 & 12.97 & 1.00 & 40.34 & 4.09 & & 1.12 & Gaia DR3 \\
91 & 07:36:20.30 & -15:11:22.1 & 13.86 & 0.99 & 30.68 & 3.32 & & 0.98 & Gaia DR3 \\
92 & 07:36:21.35 & -14:26:30.3 & 13.77 & 1.00 & 27.10 & 4.65 & & 1.08 & Gaia DR3 \\
93 & 07:36:21.64 & -14:44:26.6 & 9.11 & 1.00 & 29.67 & 3.45 & & 0.98 & Gaia DR3 \\
94 & 07:36:22.06 & -14:30:28.3 & 10.41 & 1.00 & 30.60 & 2.70 & & 0.88 & Gaia DR3 \\
95 & 07:36:22.62 & -14:29:45.5 & 8.70 & 1.00 & 37.98 & 2.59 & & 0.91 & Gaia DR3 \\
96 & 07:36:22.72 & -14:23:32.0 & 14.51 & 1.00 & 32.43 & 6.74 & & 0.96 & Gaia DR3 \\
97 & 07:36:24.35 & -14:39:57.0 & 12.54 & 1.00 & 36.56 & 12.04 & & 0.95 & Gaia DR3 \\
98 & 07:36:24.90 & -14:27:14.3 & 14.92 & 1.00 & 27.34 & 6.81 & & 1.02 & Gaia DR3 \\
99 & 07:36:25.15 & -14:32:30.2 & 12.59 & 1.00 & 37.06 & 2.16 & & 1.17 & Gaia DR3 \\
100 & 07:36:25.16 & -14:54:36.6 & 13.89 & 0.99 & 36.21 & 5.11 & & 1.10 & Gaia DR3 \\
101 & 07:36:25.23 & -14:34:35.4 & 14.84 & 1.00 & 82.16 & 8.88 & & 1.38 & Gaia DR3 \\
102 & 07:36:25.35 & -13:22:18.2 & 11.35 & 1.00 & 35.96 & 3.51 & & 1.23 & Gaia DR3 \\
103 & 07:36:25.64 & -14:11:06.4 & 14.68 & 1.00 & 29.55 & 5.54 & & 1.04 & Gaia DR3 \\
104 & 07:36:25.79 & -13:56:29.1 & 14.84 & 1.00 & 32.35 & 7.76 & & 1.00 & Gaia DR3 \\
105 & 07:36:25.79 & -14:29:07.7 & 9.43 & 1.00 & 29.14 & 5.44 & & 0.89 & Gaia DR3 \\
106 & 07:36:26.15 & -14:39:29.9 & 12.56 & 1.00 & 35.71 & 3.83 & & 0.97 & Gaia DR3 \\
107 & 07:36:27.46 & -14:38:47.2 & 11.78 & 1.00 & 30.51 & 6.06 & & 0.93 & Gaia DR3 \\
108 & 07:36:27.58 & -14:13:36.7 & 9.93 & 1.00 & 28.52 & 4.43 & & 0.82 & Gaia DR3 \\
109 & 07:36:28.53 & -14:56:54.4 & 14.78 & 1.00 & 90.66 & 8.42 & & 0.96 & Gaia DR3 \\
110 & 07:36:30.01 & -14:19:31.2 & 11.58 & 1.00 & 35.95 & 2.08 & & 0.86 & Gaia DR3 \\
111 & 07:36:31.36 & -14:00:21.1 & 11.12 & 0.99 & 35.82 & 1.48 & & 1.09 & Gaia DR3 \\
112 & 07:36:31.85 & -14:29:41.8 & 10.76 & 1.00 & 27.82 & 2.95 & & 0.97 & Gaia DR3 \\
113 & 07:36:32.11 & -14:28:04.5 & 11.41 & 1.00 & 36.60 & 10.57 & & 0.86 & Gaia DR3 \\
114 & 07:36:32.78 & -14:14:33.4 & 8.64 & 1.00 & 32.22 & 1.69 & & 0.85 & Gaia DR3 \\
115 & 07:36:34.88 & -14:25:49.0 & 8.77 & 1.00 & 34.45 & 2.29 & & 0.91 & Gaia DR3 \\
116 & 07:36:35.70 & -14:29:00.4 & 7.09 & 1.00 & 33.00 & 3.28 & & 1.00 & Gaia DR3 \\
117 & 07:36:36.00 & -14:32:37.8 & 11.49 & 1.00 & 39.53 & 2.58 & & 0.81 & Gaia DR3 \\
118 & 07:36:36.48 & -14:08:37.8 & 9.81 & 1.00 & 27.45 & 3.37 & & 0.93 & Gaia DR3 \\
119 & 07:36:37.04 & -14:30:51.7 & 12.31 & 1.00 & 29.77 & 3.94 & & 0.90 & Gaia DR3 \\
120 & 07:36:37.07 & -14:09:53.6 & 14.15 & 1.00 & 35.28 & 5.20 & & 0.98 & Gaia DR3 \\
121 & 07:36:37.63 & -14:42:13.0 & 12.67 & 1.00 & 34.55 & 4.75 & & 0.98 & Gaia DR3 \\
122 & 07:36:37.68 & -14:38:18.9 & 14.62 & 1.00 & 46.44 & 11.67 & & 1.03 & Gaia DR3 \\
123 & 07:36:38.15 & -14:41:29.3 & 13.15 & 1.00 & 38.00 & 3.35 & & 0.95 & Gaia DR3 \\
124 & 07:36:38.18 & -14:58:51.4 & 12.34 & 1.00 & 36.60 & 1.89 & & 0.87 & Gaia DR3 \\
125 & 07:36:38.64 & -14:24:48.8 & 11.65 & 1.00 & 37.08 & 2.30 & & 0.89 & Gaia DR3 \\
126 & 07:36:39.04 & -14:50:51.8 & 11.51 & 0.99 & 36.21 & 4.98 & & 0.97 & Gaia DR3 \\
127 & 07:36:39.13 & -14:37:30.8 & 12.93 & 1.00 & 34.80 & 2.35 & & 1.03 & Gaia DR3 \\
128 & 07:36:39.43 & -14:23:34.2 & 10.16 & 1.00 & 31.67 & 2.52 & & 0.81 & Gaia DR3 \\
129 & 07:36:39.54 & -14:39:14.3 & 13.68 & 1.00 & 34.22 & 2.89 & & 1.04 & Gaia DR3 \\
130 & 07:36:39.90 & -14:33:14.9 & 14.83 & 1.00 & 47.95 & 14.75 & & 1.04 & Gaia DR3 \\
131 & 07:36:40.51 & -14:29:14.8 & 9.71 & 1.00 & 37.81 & 1.89 & & 1.20 & Gaia DR3 \\
132 & 07:36:41.02 & -14:34:45.7 & 11.13 & 1.00 & 42.04 & 3.58 & & 1.02 & Gaia DR3 \\
133 & 07:36:41.25 & -14:26:37.0 & 6.67 & 1.00 & 50.24 & 3.28 & & 1.08 & Gaia DR3 \\
134 & 07:36:41.27 & -14:35:30.8 & 11.37 & 1.00 & 32.56 & 2.72 & & 0.92 & Gaia DR3 \\
135 & 07:36:42.18 & -14:32:31.1 & 11.18 & 1.00 & 29.40 & 5.11 & & 1.02 & Gaia DR3 \\
136 & 07:36:43.35 & -14:40:55.2 & 11.67 & 0.73 & 11.83 & 3.71 & & 0.99 & Gaia DR3 \\
137 & 07:36:43.74 & -14:28:46.7 & 11.64 & 1.00 & 35.90 & 1.32 & & 0.87 & Gaia DR3 \\
138 & 07:36:44.97 & -14:21:44.8 & 14.06 & 1.00 & 39.87 & 7.00 & & 0.99 & Gaia DR3 \\
139 & 07:36:45.64 & -14:28:55.3 & 12.83 & 1.00 & 31.78 & 2.85 & & 1.00 & Gaia DR3 \\
140 & 07:36:45.77 & -14:34:34.9 & 14.31 & 1.00 & 32.81 & 3.64 & & 1.01 & Gaia DR3 \\
141 & 07:36:45.80 & -15:27:45.5 & 11.36 & 1.00 & 34.04 & 3.47 & & 0.97 & Gaia DR3 \\
142 & 07:36:45.84 & -14:37:51.4 & 12.00 & 1.00 & 37.61 & 1.72 & & 0.95 & Gaia DR3 \\
143 & 07:36:46.43 & -14:21:38.8 & 13.55 & 1.00 & 34.81 & 2.47 & & 0.93 & Gaia DR3 \\
144 & 07:36:46.48 & -14:24:19.9 & 10.33 & 1.00 & 24.07 & 4.68 & & 0.96 & Gaia DR3 \\
145 & 07:36:48.62 & -14:22:25.0 & 13.90 & 1.00 & 34.05 & 4.79 & & 0.97 & Gaia DR3 \\
146 & 07:36:50.06 & -14:22:59.6 & 12.29 & 1.00 & 36.31 & 2.65 & & 0.94 & Gaia DR3 \\
147 & 07:36:51.10 & -13:24:37.0 & 12.28 & 1.00 & 36.70 & 5.08 & & 1.01 & Gaia DR3 \\
148 & 07:36:52.32 & -14:24:32.3 & 9.76 & 1.00 & 30.61 & 2.61 & & 0.93 & Gaia DR3 \\
149 & 07:36:52.57 & -14:58:34.6 & 12.49 & 1.00 & 33.48 & 4.06 & & 0.96 & Gaia DR3 \\
150 & 07:36:52.73 & -14:34:13.3 & 14.39 & 0.99 & 29.59 & 6.76 & & 1.04 & Gaia DR3 \\
151 & 07:36:53.05 & -14:33:15.7 & 10.11 & 1.00 & 23.48 & 3.31 & & 0.97 & Gaia DR3 \\
152 & 07:36:53.33 & -14:15:10.9 & 14.71 & 1.00 & 39.24 & 6.39 & & 1.04 & Gaia DR3 \\
153 & 07:36:53.88 & -14:23:30.1 & 14.59 & 1.00 & 78.66 & 8.83 & & 0.95 & Gaia DR3 \\
154 & 07:36:54.68 & -15:05:43.4 & 13.41 & 1.00 & 44.41 & 3.77 & & 1.00 & Gaia DR3 \\
155 & 07:36:54.90 & -14:30:29.9 & 13.10 & 1.00 & 33.98 & 2.97 & & 0.94 & Gaia DR3 \\
156 & 07:36:55.22 & -15:17:34.2 & 13.16 & 0.99 & 37.63 & 4.32 & & 0.98 & Gaia DR3 \\
157 & 07:36:55.25 & -14:33:17.6 & 10.68 & 0.99 & 33.45 & 1.10 & & 1.11 & Gaia DR3 \\
158 & 07:36:56.63 & -14:27:42.6 & 13.83 & 1.00 & 36.51 & 3.54 & & 0.97 & Gaia DR3 \\
159 & 07:36:57.57 & -14:50:44.6 & 13.43 & 1.00 & 36.61 & 3.62 & & 1.01 & Gaia DR3 \\
160 & 07:36:58.40 & -14:35:54.4 & 13.33 & 1.00 & 32.92 & 2.76 & & 0.95 & Gaia DR3 \\
161 & 07:36:58.61 & -14:29:54.2 & 14.36 & 0.99 & 34.24 & 4.64 & & 1.05 & Gaia DR3 \\
162 & 07:36:58.85 & -14:36:21.8 & 12.32 & 1.00 & 36.82 & 2.35 & & 1.00 & Gaia DR3 \\
163 & 07:36:59.02 & -13:56:16.9 & 12.15 & 1.00 & 37.56 & 5.44 & & 0.99 & Gaia DR3 \\
164 & 07:36:59.59 & -14:55:53.2 & 14.54 & 1.00 & 31.52 & 6.94 & & 1.02 & Gaia DR3 \\
165 & 07:37:00.32 & -14:26:03.3 & 13.17 & 1.00 & 40.14 & 2.65 & & 0.97 & Gaia DR3 \\
166 & 07:37:01.01 & -14:39:34.4 & 11.16 & 1.00 & 35.52 & 1.19 & & 0.89 & Gaia DR3 \\
167 & 07:37:02.36 & -14:31:13.6 & 11.09 & 1.00 & 36.68 & 1.46 & & 0.89 & Gaia DR3 \\
168 & 07:37:03.97 & -15:19:23.5 & 10.19 & 0.94 & 26.96 & 3.32 & & 1.03 & Gaia DR3 \\
169 & 07:37:04.89 & -14:45:24.2 & 14.80 & 0.99 & 38.69 & 5.37 & & 1.01 & Gaia DR3 \\
170 & 07:37:05.66 & -14:24:24.5 & 10.32 & 1.00 & 22.31 & 5.68 & & 0.86 & Gaia DR3 \\
171 & 07:37:06.63 & -14:31:45.6 & 12.39 & 1.00 & 38.48 & 12.46 & & 0.95 & Gaia DR3 \\
172 & 07:37:07.17 & -14:15:42.5 & 12.36 & 1.00 & 37.29 & 29.21 & & 0.91 & Gaia DR3 \\
173 & 07:37:08.00 & -14:04:16.7 & 14.61 & 1.00 & 35.89 & 14.19 & & 1.20 & Gaia DR3 \\
174 & 07:37:08.26 & -14:33:14.7 & 10.48 & 1.00 & 30.71 & 1.32 & & 1.34 & RAVE \\
175 & 07:37:09.83 & -14:24:54.3 & 15.01 & 0.97 & 71.09 & 11.35 & & 1.08 & Gaia DR3 \\
176 & 07:37:10.52 & -14:33:41.5 & 11.70 & 1.00 & 40.52 & 3.35 & & 0.89 & Gaia DR3 \\
177 & 07:37:11.38 & -14:15:57.5 & 11.41 & 1.00 & 35.31 & 2.15 & & 0.94 & Gaia DR3 \\
178 & 07:37:13.11 & -14:29:11.8 & 11.26 & 1.00 & 33.65 & 1.31 & & 0.99 & Gaia DR3 \\
179 & 07:37:14.50 & -14:25:18.0 & 9.95 & 1.00 & 29.51 & 4.60 & & 0.94 & Gaia DR3 \\
180 & 07:37:14.82 & -14:32:14.9 & 12.06 & 1.00 & 37.33 & 4.00 & & 0.89 & Gaia DR3 \\
181 & 07:37:15.28 & -14:25:56.7 & 11.91 & 1.00 & 26.30 & 4.12 & & 0.99 & Gaia DR3 \\
182 & 07:37:15.40 & -14:33:35.6 & 13.32 & 1.00 & 31.86 & 6.25 & & 1.00 & Gaia DR3 \\
183 & 07:37:15.56 & -14:31:48.8 & 12.40 & 1.00 & 31.79 & 3.55 & & 1.03 & Gaia DR3 \\
184 & 07:37:18.22 & -14:32:45.7 & 14.93 & 1.00 & 24.60 & 8.43 & & 0.96 & Gaia DR3 \\
185 & 07:37:22.30 & -14:29:41.4 & 14.82 & 1.00 & 38.57 & 6.72 & & 1.30 & Gaia DR3 \\
186 & 07:37:22.52 & -14:35:49.7 & 10.72 & 1.00 & 18.43 & 5.78 & & 0.99 & RAVE \\
187 & 07:37:23.29 & -14:25:11.6 & 12.94 & 1.00 & 35.84 & 2.18 & & 0.94 & Gaia DR3 \\
188 & 07:37:24.69 & -14:23:36.7 & 11.94 & 1.00 & 34.40 & 6.47 & & 0.97 & Gaia DR3 \\
189 & 07:37:27.21 & -14:17:12.9 & 14.36 & 0.99 & -5.14 & 5.94 & & 0.96 & Gaia DR3 \\
190 & 07:37:27.91 & -14:25:17.6 & 12.89 & 1.00 & 33.18 & 2.38 & & 1.04 & Gaia DR3 \\
191 & 07:37:31.09 & -14:18:00.1 & 12.71 & 1.00 & 32.40 & 5.38 & & 1.02 & Gaia DR3 \\
192 & 07:37:32.91 & -14:29:19.4 & 14.79 & 1.00 & 41.03 & 6.76 & & 1.00 & Gaia DR3 \\
193 & 07:37:34.84 & -14:24:29.4 & 11.64 & 1.00 & 39.13 & 2.84 & & 0.99 & Gaia DR3 \\
194 & 07:37:35.05 & -14:04:26.3 & 13.97 & 1.00 & 30.80 & 4.18 & & 0.97 & Gaia DR3 \\
195 & 07:37:37.11 & -14:25:25.5 & 8.90 & 1.00 & 31.42 & 2.98 & & 0.85 & Gaia DR3 \\
196 & 07:37:37.73 & -14:27:49.8 & 10.92 & 1.00 & 30.44 & 3.32 & & 1.27 & RAVE \\
197 & 07:37:38.80 & -14:26:26.7 & 6.49 & 1.00 & 69.56 & 0.66 & & 0.96 & Gaia DR3 \\
198 & 07:37:38.99 & -14:40:05.2 & 13.44 & 1.00 & 27.43 & 5.23 & & 1.05 & Gaia DR3 \\
199 & 07:37:39.18 & -14:02:02.6 & 10.51 & 1.00 & 33.30 & 1.08 & & 0.96 & Gaia DR3 \\
200 & 07:37:43.01 & -13:55:25.5 & 11.73 & 1.00 & 38.38 & 6.72 & & 0.95 & Gaia DR3 \\
201 & 07:37:45.81 & -14:35:47.7 & 10.72 & 1.00 & 28.35 & 7.08 & & 0.94 & Gaia DR3 \\
202 & 07:37:46.02 & -13:40:13.0 & 11.81 & 1.00 & 25.47 & 9.17 & & 0.97 & Gaia DR3 \\
203 & 07:37:46.32 & -14:36:38.8 & 14.24 & 1.00 & 9.25 & 5.14 & & 1.10 & Gaia DR3 \\
204 & 07:37:47.34 & -14:15:39.7 & 14.69 & 1.00 & 33.71 & 8.40 & & 1.04 & Gaia DR3 \\
205 & 07:37:48.62 & -14:30:29.1 & 11.67 & 1.00 & 37.01 & 1.01 & & 1.04 & Gaia DR3 \\
206 & 07:37:58.26 & -14:21:49.0 & 14.09 & 1.00 & 37.44 & 4.50 & & 0.99 & Gaia DR3 \\
207 & 07:37:58.94 & -15:05:45.4 & 13.27 & 0.99 & 34.54 & 2.62 & & 1.01 & Gaia DR3 \\
208 & 07:37:59.99 & -14:48:18.0 & 13.37 & 1.00 & 38.08 & 6.43 & & 0.95 & Gaia DR3 \\
209 & 07:38:01.11 & -13:43:34.5 & 10.01 & 0.98 & 23.01 & 4.25 & & 0.88 & Gaia DR3 \\
210 & 07:38:03.84 & -13:44:04.6 & 10.09 & 0.83 & 27.05 & 2.47 & & 0.95 & Gaia DR3 \\
211 & 07:38:05.72 & -15:06:17.8 & 14.30 & 0.99 & 33.22 & 4.38 & & 0.97 & Gaia DR3 \\
212 & 07:38:07.82 & -14:12:09.8 & 14.96 & 1.00 & 16.05 & 9.96 & & 1.00 & Gaia DR3 \\
213 & 07:38:13.75 & -14:14:24.7 & 13.71 & 0.98 & 33.94 & 5.73 & & 1.04 & Gaia DR3 \\
214 & 07:38:14.46 & -14:26:55.1 & 13.79 & 1.00 & 33.94 & 2.77 & & 1.01 & Gaia DR3 \\
215 & 07:38:14.60 & -14:04:59.0 & 10.95 & 1.00 & 34.53 & 8.25 & & 1.26 & Gaia DR3 \\
216 & 07:38:24.83 & -14:18:49.2 & 12.47 & 1.00 & 25.66 & 4.60 & & 0.91 & Gaia DR3 \\
217 & 07:38:26.53 & -14:21:04.1 & 14.42 & 1.00 & 35.59 & 4.38 & & 1.01 & Gaia DR3 \\
218 & 07:38:31.42 & -14:35:42.0 & 12.09 & 1.00 & 35.86 & 0.80 & & 0.91 & Gaia DR3 \\
219 & 07:38:35.64 & -14:29:53.9 & 11.03 & 1.00 & 34.67 & 5.48 & & 0.99 & RAVE \\
220 & 07:38:42.44 & -14:24:16.6 & 12.68 & 0.99 & 34.18 & 4.67 & & 0.90 & Gaia DR3 \\
221 & 07:38:55.93 & -14:55:42.6 & 14.02 & 0.99 & 44.45 & 4.76 & & 1.01 & Gaia DR3 \\
222 & 07:39:03.66 & -14:13:46.9 & 12.88 & 0.99 & 38.92 & 3.41 & & 0.92 & Gaia DR3 \\
223 & 07:39:17.78 & -14:20:45.4 & 14.62 & 0.98 & 32.82 & 4.71 & & 1.03 & Gaia DR3 \\
224 & 07:39:20.99 & -13:26:44.5 & 9.69 & 0.63 & 21.64 & 16.04 & & 1.04 & Gaia DR3 \\
225 & 07:39:25.52 & -15:06:48.3 & 10.80 & 0.97 & 22.98 & 6.33 & & 1.12 & Gaia DR3 \\
226 & 07:39:32.92 & -13:59:10.9 & 14.14 & 0.98 & 34.99 & 6.11 & & 0.97 & Gaia DR3 \\
227 & 07:39:34.08 & -14:09:06.1 & 9.36 & 0.99 & 31.23 & 3.52 & & 1.03 & Gaia DR3 \\
228 & 07:39:37.11 & -14:51:41.5 & 14.68 & 0.97 & 29.44 & 5.41 & & 0.97 & Gaia DR3 \\
229 & 07:39:57.15 & -13:50:46.6 & 13.11 & 1.00 & 36.18 & 2.20 & & 0.96 & Gaia DR3 \\
230 & 07:40:46.53 & -14:30:48.2 & 9.90 & 0.88 & 19.31 & 4.90 & & 0.92 & Gaia DR3 \\
231 & 07:41:03.37 & -14:34:07.2 & 10.14 & 0.73 & 30.82 & 6.03 & & 0.93 & Gaia DR3 \\
\hline
\end{tabular}
\label{tab:NGC_2422}
\end{table*}


% Tablo: NGC_2437
\begin{table*} \footnotesize
\centering
\caption{Radial velocity measurements for NGC 2437}
\begin{tabular}{l c c c c c c c c l}
\hline\hline
ID & $\alpha$ (hh:mm:ss) & $\delta$ (dd:mm:ss) & $G$ (mag) & $P$ & $V_R$ (km s$^{-1}$)& $\sigma_{V_R}$ & & RUWE & Survey \\
\hline
1 & 07:39:36.19 & -14:40:19.3 & 14.40 & 0.73 & 71.66 & 28.70 & & 1.09 & Gaia DR3 \\
2 & 07:39:57.78 & -14:51:27.5 & 11.24 & 0.87 & 50.42 & 6.39 & & 0.95 & Gaia DR3 \\
3 & 07:40:22.56 & -14:39:06.3 & 11.77 & 1.00 & 33.70 & 6.71 & & 0.94 & Gaia DR3 \\
4 & 07:40:25.60 & -14:22:08.2 & 14.13 & 0.66 & 47.90 & 14.69 & & 1.01 & Gaia DR3 \\
5 & 07:40:26.09 & -14:48:00.7 & 11.71 & 0.91 & 46.57 & 11.08 & & 0.88 & Gaia DR3 \\
6 & 07:40:28.33 & -14:48:52.6 & 14.73 & 0.95 & 46.18 & 8.74 & & 1.04 & Gaia DR3 \\
7 & 07:40:29.73 & -15:13:03.5 & 12.29 & 0.83 & 55.23 & 11.57 & & 1.24 & Gaia DR3 \\
8 & 07:40:30.48 & -14:34:29.9 & 14.56 & 0.94 & 55.79 & 26.75 & & 1.00 & Gaia DR3 \\
9 & 07:40:38.13 & -14:26:37.3 & 11.81 & 0.86 & 27.76 & 16.80 & & 0.88 & Gaia DR3 \\
10 & 07:40:38.32 & -14:26:23.2 & 14.59 & 0.89 & 87.79 & 10.04 & & 1.01 & Gaia DR3 \\
11 & 07:40:43.08 & -14:53:08.0 & 14.28 & 0.99 & 51.32 & 10.10 & & 1.03 & Gaia DR3 \\
12 & 07:40:44.32 & -15:05:59.4 & 14.58 & 0.95 & 42.62 & 11.19 & & 0.96 & Gaia DR3 \\
13 & 07:40:45.15 & -14:39:57.6 & 11.91 & 0.98 & 62.17 & 20.45 & & 0.96 & Gaia DR3 \\
14 & 07:40:46.38 & -15:17:08.5 & 14.54 & 0.78 & 31.18 & 36.97 & & 0.99 & Gaia DR3 \\
15 & 07:40:47.61 & -14:45:57.3 & 11.14 & 1.00 & 49.09 & 0.50 & & 1.08 & Gaia DR3 \\
16 & 07:40:51.52 & -14:47:26.2 & 14.52 & 0.99 & 47.32 & 13.14 & & 1.01 & Gaia DR3 \\
17 & 07:40:54.69 & -14:22:07.0 & 10.92 & 0.87 & 33.47 & 5.02 & & 0.98 & Gaia DR3 \\
18 & 07:40:58.03 & -14:51:02.6 & 12.02 & 1.00 & 33.56 & 16.43 & & 0.89 & Gaia DR3 \\
19 & 07:40:59.49 & -14:43:59.9 & 13.93 & 0.99 & 39.19 & 11.74 & & 0.99 & Gaia DR3 \\
20 & 07:41:00.64 & -14:22:17.3 & 10.42 & 1.00 & 48.26 & 0.19 & & 1.00 & Gaia DR3 \\
21 & 07:41:02.54 & -14:47:47.4 & 10.77 & 1.00 & 46.94 & 4.18 & & 0.98 & Gaia DR3 \\
22 & 07:41:08.71 & -14:51:29.4 & 14.46 & 0.99 & 45.88 & 7.53 & & 1.08 & Gaia DR3 \\
23 & 07:41:11.13 & -14:39:54.0 & 11.01 & 0.98 & 43.55 & 3.19 & & 1.04 & Gaia DR3 \\
24 & 07:41:11.27 & -14:52:28.1 & 11.64 & 0.99 & 41.83 & 11.29 & & 0.83 & Gaia DR3 \\
25 & 07:41:11.90 & -15:01:39.3 & 11.99 & 0.99 & 37.49 & 12.64 & & 0.93 & Gaia DR3 \\
26 & 07:41:16.18 & -14:56:18.7 & 14.36 & 0.96 & 39.52 & 7.81 & & 1.00 & Gaia DR3 \\
27 & 07:41:16.86 & -14:32:56.8 & 14.23 & 0.95 & 7.07 & 18.20 & & 0.91 & Gaia DR3 \\
28 & 07:41:17.10 & -14:47:30.0 & 11.91 & 0.97 & 60.18 & 17.01 & & 0.86 & Gaia DR3 \\
29 & 07:41:17.35 & -14:51:23.0 & 14.39 & 0.70 & 43.12 & 8.62 & & 1.01 & Gaia DR3 \\
30 & 07:41:17.40 & -14:49:24.7 & 14.54 & 1.00 & 75.44 & 8.85 & & 0.95 & Gaia DR3 \\
31 & 07:41:19.43 & -14:48:47.5 & 9.88 & 1.00 & 53.63 & 4.96 & & 1.10 & Gaia DR3 \\
32 & 07:41:19.96 & -14:54:22.9 & 10.60 & 1.00 & 51.65 & 3.80 & & 1.17 & Gaia DR3 \\
33 & 07:41:21.31 & -14:38:17.5 & 11.04 & 1.00 & 48.33 & 0.29 & & 0.96 & Gaia DR3 \\
34 & 07:41:22.03 & -14:57:42.6 & 14.15 & 0.99 & 38.12 & 9.99 & & 0.94 & Gaia DR3 \\
35 & 07:41:22.90 & -14:49:11.1 & 8.63 & 0.97 & 44.01 & 0.98 & & 1.05 & Gaia DR3 \\
36 & 07:41:23.53 & -14:45:53.8 & 10.26 & 1.00 & 46.82 & 2.04 & & 1.14 & Gaia DR3 \\
37 & 07:41:24.21 & -15:06:29.7 & 14.52 & 0.99 & 57.87 & 10.88 & & 1.01 & Gaia DR3 \\
38 & 07:41:25.93 & -14:41:13.6 & 11.30 & 0.95 & 45.79 & 6.74 & & 1.16 & Gaia DR3 \\
39 & 07:41:26.73 & -14:34:57.1 & 14.48 & 0.98 & 91.19 & 17.63 & & 0.96 & Gaia DR3 \\
40 & 07:41:27.44 & -14:41:13.7 & 14.63 & 1.00 & 21.41 & 12.05 & & 0.96 & Gaia DR3 \\
41 & 07:41:27.84 & -14:51:54.0 & 11.43 & 1.00 & 32.47 & 27.15 & & 0.99 & Gaia DR3 \\
42 & 07:41:28.19 & -14:45:40.1 & 12.02 & 0.96 & 76.11 & 20.16 & & 0.90 & Gaia DR3 \\
43 & 07:41:28.53 & -14:54:17.4 & 10.30 & 0.99 & 42.60 & 2.37 & & 1.25 & Gaia DR3 \\
44 & 07:41:28.97 & -14:47:36.5 & 10.71 & 1.00 & 68.37 & 12.85 & & 0.93 & Gaia DR3 \\
45 & 07:41:29.35 & -14:47:18.8 & 14.53 & 1.00 & 79.20 & 12.54 & & 1.00 & Gaia DR3 \\
46 & 07:41:29.66 & -14:48:59.8 & 11.99 & 0.99 & 53.87 & 22.25 & & 0.91 & Gaia DR3 \\
47 & 07:41:29.97 & -14:47:09.3 & 12.19 & 0.99 & 101.98 & 21.59 & & 1.26 & Gaia DR3 \\
48 & 07:41:30.00 & -14:53:20.4 & 11.24 & 0.99 & 24.26 & 7.26 & & 1.14 & Gaia DR3 \\
49 & 07:41:30.55 & -14:52:59.1 & 14.34 & 1.00 & 50.49 & 8.45 & & 1.23 & Gaia DR3 \\
50 & 07:41:30.55 & -14:53:53.9 & 11.24 & 1.00 & 47.67 & 9.25 & & 1.10 & RAVE \\
51 & 07:41:30.90 & -14:56:22.0 & 11.47 & 0.97 & 45.22 & 6.99 & & 0.78 & Gaia DR3 \\
52 & 07:41:31.39 & -14:20:47.4 & 14.09 & 0.88 & 43.68 & 11.76 & & 1.03 & Gaia DR3 \\
53 & 07:41:31.71 & -15:02:37.1 & 11.51 & 1.00 & 48.44 & 8.65 & & 0.91 & Gaia DR3 \\
54 & 07:41:32.00 & -14:51:48.4 & 10.78 & 0.99 & 54.59 & 4.41 & & 1.08 & Gaia DR3 \\
55 & 07:41:32.05 & -14:57:37.0 & 14.45 & 0.95 & 32.16 & 10.81 & & 0.97 & Gaia DR3 \\
56 & 07:41:32.64 & -14:50:58.4 & 11.76 & 1.00 & 17.88 & 17.66 & & 0.97 & Gaia DR3 \\
57 & 07:41:33.13 & -14:50:12.8 & 11.91 & 1.00 & 21.49 & 17.26 & & 0.83 & Gaia DR3 \\
58 & 07:41:33.16 & -14:40:33.9 & 14.52 & 0.99 & 45.66 & 12.26 & & 1.04 & Gaia DR3 \\
59 & 07:41:33.19 & -14:47:41.7 & 11.74 & 1.00 & 26.12 & 16.69 & & 0.98 & Gaia DR3 \\
60 & 07:41:34.67 & -14:51:31.0 & 10.41 & 1.00 & 50.01 & 2.50 & & 1.01 & Gaia DR3 \\
61 & 07:41:35.23 & -14:45:49.0 & 11.01 & 1.00 & 43.11 & 7.06 & & 0.94 & Gaia DR3 \\
62 & 07:41:35.66 & -15:05:09.8 & 14.55 & 0.80 & 43.80 & 17.80 & & 0.97 & Gaia DR3 \\
63 & 07:41:35.67 & -14:54:27.0 & 14.45 & 0.99 & 4.82 & 19.67 & & 1.03 & Gaia DR3 \\
64 & 07:41:36.88 & -15:22:19.6 & 13.78 & 0.73 & 23.95 & 4.61 & & 1.07 & Gaia DR3 \\
65 & 07:41:36.90 & -14:26:11.2 & 10.28 & 1.00 & 49.64 & 0.18 & & 0.97 & Gaia DR3 \\
66 & 07:41:37.26 & -14:49:31.1 & 12.04 & 0.99 & 41.39 & 22.98 & & 1.00 & Gaia DR3 \\
67 & 07:41:37.83 & -14:48:20.2 & 12.01 & 1.00 & 23.76 & 33.30 & & 0.97 & Gaia DR3 \\
68 & 07:41:38.71 & -14:49:07.9 & 11.74 & 1.00 & 39.56 & 12.44 & & 1.09 & Gaia DR3 \\
69 & 07:41:38.97 & -14:40:55.7 & 11.54 & 1.00 & 41.44 & 7.34 & & 1.08 & RAVE \\
70 & 07:41:40.01 & -14:44:13.9 & 11.88 & 0.99 & 37.81 & 11.97 & & 1.26 & Gaia DR3 \\
71 & 07:41:40.07 & -14:59:34.3 & 14.58 & 1.00 & 40.92 & 25.68 & & 0.95 & Gaia DR3 \\
72 & 07:41:40.18 & -14:59:26.7 & 14.42 & 0.98 & 9.50 & 15.58 & & 1.09 & Gaia DR3 \\
73 & 07:41:40.70 & -14:48:02.0 & 11.39 & 1.00 & 48.80 & 11.74 & & 1.02 & Gaia DR3 \\
74 & 07:41:41.31 & -14:39:53.2 & 11.33 & 1.00 & 45.71 & 8.09 & & 0.96 & Gaia DR3 \\
75 & 07:41:41.41 & -14:47:48.5 & 11.65 & 1.00 & 77.44 & 19.50 & & 0.88 & Gaia DR3 \\
76 & 07:41:41.95 & -14:47:15.8 & 11.29 & 0.99 & 45.42 & 10.89 & & 1.08 & Gaia DR3 \\
77 & 07:41:42.12 & -14:53:32.0 & 14.59 & 0.97 & 78.68 & 19.28 & & 0.97 & Gaia DR3 \\
78 & 07:41:42.14 & -14:45:44.3 & 14.39 & 0.99 & 33.69 & 25.18 & & 1.03 & Gaia DR3 \\
79 & 07:41:42.86 & -14:57:02.3 & 11.08 & 0.99 & 35.76 & 5.12 & & 0.87 & Gaia DR3 \\
80 & 07:41:43.60 & -14:58:29.5 & 11.13 & 1.00 & 52.39 & 3.97 & & 0.93 & Gaia DR3 \\
81 & 07:41:43.96 & -15:00:21.1 & 14.56 & 1.00 & 33.75 & 11.54 & & 0.86 & Gaia DR3 \\
82 & 07:41:44.53 & -15:16:00.8 & 14.17 & 0.91 & 52.74 & 11.72 & & 0.93 & Gaia DR3 \\
83 & 07:41:44.92 & -14:58:35.0 & 14.54 & 0.99 & 42.82 & 8.56 & & 1.01 & Gaia DR3 \\
84 & 07:41:45.12 & -14:50:02.0 & 11.18 & 0.99 & 47.85 & 14.57 & & 1.06 & Gaia DR3 \\
85 & 07:41:45.14 & -14:50:00.0 & 11.84 & 1.00 & -1.41 & 25.07 & & 1.04 & Gaia DR3 \\
86 & 07:41:45.28 & -15:05:26.3 & 14.49 & 0.97 & 26.30 & 11.87 & & 1.07 & Gaia DR3 \\
87 & 07:41:45.73 & -14:50:36.9 & 13.96 & 1.00 & 15.74 & 6.60 & & 0.92 & Gaia DR3 \\
88 & 07:41:48.51 & -14:53:55.9 & 11.93 & 0.99 & 54.35 & 19.57 & & 1.13 & Gaia DR3 \\
89 & 07:41:48.56 & -14:53:02.0 & 10.63 & 0.99 & 48.20 & 1.86 & & 0.91 & Gaia DR3 \\
90 & 07:41:49.02 & -14:28:30.3 & 11.52 & 1.00 & 46.00 & 9.30 & & 1.25 & Gaia DR3 \\
91 & 07:41:49.14 & -14:46:56.2 & 11.16 & 1.00 & 37.48 & 9.09 & & 1.02 & Gaia DR3 \\
92 & 07:41:49.86 & -14:51:15.1 & 10.54 & 1.00 & 35.14 & 6.74 & & 0.90 & Gaia DR3 \\
93 & 07:41:49.91 & -14:45:19.8 & 12.16 & 1.00 & 32.69 & 18.21 & & 0.97 & Gaia DR3 \\
94 & 07:41:50.15 & -14:32:34.1 & 10.94 & 0.98 & 58.39 & 6.56 & & 1.03 & Gaia DR3 \\
95 & 07:41:50.63 & -14:40:07.8 & 11.85 & 0.99 & 43.54 & 13.14 & & 0.89 & Gaia DR3 \\
96 & 07:41:51.53 & -14:54:29.2 & 10.30 & 1.00 & 46.50 & 0.28 & & 0.92 & Gaia DR3 \\
97 & 07:41:51.53 & -14:49:00.1 & 11.57 & 1.00 & 46.29 & 22.48 & & 0.95 & Gaia DR3 \\
98 & 07:41:51.65 & -14:47:11.0 & 11.54 & 1.00 & 52.42 & 17.84 & & 1.03 & Gaia DR3 \\
99 & 07:41:51.93 & -14:46:49.5 & 10.90 & 1.00 & 48.81 & 9.78 & & 1.05 & Gaia DR3 \\
100 & 07:41:52.48 & -15:10:41.2 & 14.40 & 0.94 & 17.58 & 10.50 & & 1.01 & Gaia DR3 \\
101 & 07:41:52.56 & -15:04:30.7 & 14.62 & 0.99 & 22.28 & 11.14 & & 1.03 & Gaia DR3 \\
102 & 07:41:52.56 & -14:52:14.1 & 11.51 & 1.00 & 46.44 & 32.26 & & 1.11 & Gaia DR3 \\
103 & 07:41:52.77 & -14:47:46.1 & 12.13 & 1.00 & 51.81 & 22.93 & & 0.94 & Gaia DR3 \\
104 & 07:41:52.91 & -14:44:32.3 & 11.28 & 1.00 & 40.54 & 10.63 & & 0.99 & Gaia DR3 \\
105 & 07:41:53.43 & -14:45:43.0 & 14.22 & 1.00 & 41.13 & 7.39 & & 1.05 & Gaia DR3 \\
106 & 07:41:54.27 & -14:57:20.6 & 11.94 & 1.00 & 37.88 & 15.30 & & 0.92 & Gaia DR3 \\
107 & 07:41:54.49 & -14:50:11.6 & 11.25 & 1.00 & 45.31 & 11.53 & & 1.33 & Gaia DR3 \\
108 & 07:41:54.50 & -15:05:15.2 & 11.65 & 1.00 & 47.07 & 8.43 & & 0.93 & RAVE \\
109 & 07:41:55.76 & -14:56:34.8 & 11.82 & 1.00 & 31.15 & 13.66 & & 0.82 & Gaia DR3 \\
110 & 07:41:57.04 & -14:25:44.8 & 14.30 & 0.92 & 107.20 & 14.63 & & 0.96 & Gaia DR3 \\
111 & 07:41:57.32 & -14:30:28.4 & 14.42 & 0.97 & 49.87 & 18.80 & & 0.97 & Gaia DR3 \\
112 & 07:41:58.01 & -14:59:26.0 & 12.02 & 1.00 & 54.16 & 16.62 & & 0.84 & Gaia DR3 \\
113 & 07:41:58.39 & -14:45:27.6 & 14.45 & 0.93 & 88.70 & 10.57 & & 0.97 & Gaia DR3 \\
114 & 07:41:58.43 & -14:49:24.8 & 10.25 & 0.99 & 57.35 & 2.68 & & 0.92 & Gaia DR3 \\
115 & 07:42:00.54 & -14:27:27.7 & 14.55 & 0.94 & 53.98 & 23.28 & & 0.98 & Gaia DR3 \\
116 & 07:42:02.55 & -14:46:26.8 & 11.77 & 0.99 & 40.33 & 10.51 & & 0.99 & Gaia DR3 \\
117 & 07:42:02.98 & -14:45:03.0 & 11.31 & 0.98 & 49.98 & 6.82 & & 0.94 & Gaia DR3 \\
118 & 07:42:03.02 & -14:43:43.3 & 12.10 & 1.00 & 44.69 & 9.38 & & 0.92 & Gaia DR3 \\
119 & 07:42:03.12 & -14:53:02.7 & 10.29 & 1.00 & 44.62 & 2.51 & & 0.96 & Gaia DR3 \\
120 & 07:42:03.51 & -14:55:41.7 & 11.73 & 0.85 & 55.39 & 26.82 & & 0.86 & Gaia DR3 \\
121 & 07:42:03.55 & -14:50:39.4 & 14.44 & 1.00 & 59.03 & 17.08 & & 1.00 & Gaia DR3 \\
122 & 07:42:04.35 & -14:57:08.2 & 11.43 & 1.00 & 41.47 & 10.31 & & 0.85 & RAVE \\
123 & 07:42:05.75 & -15:07:16.2 & 14.52 & 0.99 & 57.36 & 12.98 & & 1.01 & Gaia DR3 \\
124 & 07:42:05.93 & -14:44:33.6 & 10.54 & 1.00 & 49.82 & 1.20 & & 0.96 & Gaia DR3 \\
125 & 07:42:08.78 & -14:36:59.2 & 13.93 & 0.98 & 65.51 & 7.65 & & 0.98 & Gaia DR3 \\
126 & 07:42:08.90 & -14:51:04.0 & 11.74 & 1.00 & 39.50 & 19.23 & & 0.88 & RAVE \\
127 & 07:42:10.14 & -14:38:51.2 & 10.91 & 0.99 & 49.41 & 5.55 & & 1.18 & Gaia DR3 \\
128 & 07:42:10.31 & -14:47:13.1 & 11.02 & 0.99 & 41.06 & 3.35 & & 1.08 & Gaia DR3 \\
129 & 07:42:10.68 & -14:41:12.0 & 14.54 & 0.99 & 54.92 & 10.16 & & 0.98 & Gaia DR3 \\
130 & 07:42:10.73 & -14:30:59.3 & 11.09 & 1.00 & 38.44 & 6.35 & & 1.01 & Gaia DR3 \\
131 & 07:42:11.40 & -14:46:42.0 & 14.08 & 0.99 & 33.88 & 22.88 & & 1.10 & Gaia DR3 \\
132 & 07:42:11.92 & -14:48:06.2 & 14.05 & 0.98 & -38.86 & 33.83 & & 1.38 & Gaia DR3 \\
133 & 07:42:12.25 & -14:44:20.2 & 11.84 & 1.00 & 52.15 & 20.97 & & 0.98 & Gaia DR3 \\
134 & 07:42:12.90 & -14:55:18.0 & 11.85 & 1.00 & 54.23 & 11.76 & & 0.82 & Gaia DR3 \\
135 & 07:42:13.91 & -14:44:40.4 & 14.32 & 0.99 & 52.38 & 19.75 & & 1.25 & Gaia DR3 \\
136 & 07:42:16.15 & -14:49:44.4 & 10.58 & 1.00 & 47.42 & 1.21 & & 1.04 & Gaia DR3 \\
137 & 07:42:16.74 & -14:28:27.9 & 14.38 & 0.92 & 59.86 & 10.11 & & 1.06 & Gaia DR3 \\
138 & 07:42:17.59 & -14:56:09.8 & 10.93 & 1.00 & 46.66 & 6.27 & & 1.01 & RAVE \\
139 & 07:42:20.34 & -14:58:59.0 & 13.49 & 0.98 & 45.57 & 10.48 & & 1.05 & Gaia DR3 \\
140 & 07:42:21.54 & -14:27:24.5 & 14.29 & 0.79 & 63.53 & 13.18 & & 1.01 & Gaia DR3 \\
141 & 07:42:22.57 & -14:50:53.9 & 14.30 & 0.99 & 68.24 & 14.05 & & 1.06 & Gaia DR3 \\
142 & 07:42:23.88 & -15:17:44.3 & 10.84 & 1.00 & 48.69 & 0.21 & & 1.03 & Gaia DR3 \\
143 & 07:42:25.46 & -14:14:56.0 & 13.97 & 0.69 & 47.63 & 9.18 & & 0.94 & Gaia DR3 \\
144 & 07:42:25.68 & -15:20:05.6 & 11.47 & 0.88 & 51.17 & 11.62 & & 0.79 & Gaia DR3 \\
145 & 07:42:26.22 & -14:51:30.4 & 11.19 & 1.00 & 34.83 & 5.87 & & 1.06 & RAVE \\
146 & 07:42:26.39 & -14:26:20.2 & 10.94 & 0.90 & 56.10 & 9.15 & & 1.04 & Gaia DR3 \\
147 & 07:42:26.59 & -14:51:02.4 & 14.38 & 1.00 & 48.36 & 14.70 & & 1.05 & Gaia DR3 \\
148 & 07:42:30.32 & -14:57:12.2 & 12.19 & 0.99 & 35.84 & 27.67 & & 1.09 & Gaia DR3 \\
149 & 07:42:31.50 & -14:36:53.1 & 13.71 & 0.97 & 52.71 & 10.94 & & 0.94 & Gaia DR3 \\
150 & 07:42:31.53 & -14:45:47.0 & 14.32 & 0.99 & 45.62 & 10.30 & & 1.00 & Gaia DR3 \\
151 & 07:42:33.95 & -15:03:32.7 & 14.43 & 0.95 & 17.58 & 9.35 & & 0.99 & Gaia DR3 \\
152 & 07:42:34.06 & -14:49:42.9 & 14.15 & 0.99 & -49.55 & 15.61 & & 0.94 & Gaia DR3 \\
153 & 07:42:35.36 & -15:02:48.6 & 11.65 & 1.00 & 45.26 & 10.70 & & 1.01 & Gaia DR3 \\
154 & 07:42:41.24 & -14:59:51.4 & 10.95 & 1.00 & 48.65 & 0.29 & & 0.99 & Gaia DR3 \\
155 & 07:42:41.67 & -15:18:23.3 & 11.03 & 0.86 & 47.90 & 3.10 & & 0.89 & Gaia DR3 \\
156 & 07:42:44.98 & -14:39:10.5 & 14.38 & 0.96 & 54.83 & 8.97 & & 1.04 & Gaia DR3 \\
157 & 07:42:48.31 & -15:02:11.6 & 14.30 & 0.97 & 63.27 & 8.68 & & 0.97 & Gaia DR3 \\
158 & 07:42:51.31 & -14:49:14.8 & 14.49 & 0.99 & 34.66 & 8.86 & & 0.95 & Gaia DR3 \\
159 & 07:42:51.81 & -14:44:11.7 & 10.67 & 1.00 & 34.51 & 4.08 & & 1.18 & RAVE \\
160 & 07:42:56.74 & -14:39:40.9 & 13.93 & 0.92 & 57.56 & 12.90 & & 0.98 & Gaia DR3 \\
161 & 07:42:58.08 & -15:10:13.7 & 11.20 & 0.89 & 44.47 & 5.22 & & 1.28 & Gaia DR3 \\
162 & 07:42:58.97 & -14:54:53.1 & 14.50 & 0.82 & 40.87 & 15.52 & & 1.03 & Gaia DR3 \\
163 & 07:42:59.19 & -14:52:55.6 & 11.88 & 0.97 & 48.76 & 13.06 & & 0.94 & Gaia DR3 \\
164 & 07:43:04.47 & -14:59:50.1 & 14.39 & 0.95 & 64.06 & 10.13 & & 0.97 & Gaia DR3 \\
165 & 07:43:13.79 & -14:29:59.9 & 10.64 & 0.64 & 39.15 & 3.92 & & 1.17 & Gaia DR3 \\
166 & 07:43:15.04 & -14:58:32.1 & 11.49 & 0.91 & 68.72 & 15.05 & & 1.03 & Gaia DR3 \\
167 & 07:43:16.11 & -14:36:46.8 & 14.33 & 0.88 & 55.20 & 15.14 & & 1.00 & Gaia DR3 \\
168 & 07:43:16.14 & -14:52:30.2 & 11.48 & 0.66 & 43.12 & 9.95 & & 1.40 & Gaia DR3 \\
169 & 07:43:26.11 & -15:01:25.8 & 14.33 & 0.86 & 39.70 & 11.14 & & 1.02 & Gaia DR3 \\
170 & 07:43:37.56 & -14:55:50.8 & 11.77 & 0.84 & 42.55 & 32.81 & & 0.96 & Gaia DR3 \\
171 & 07:43:38.97 & -14:49:20.5 & 12.06 & 0.84 & 40.80 & 22.38 & & 0.93 & Gaia DR3 \\
172 & 07:43:40.61 & -14:30:49.5 & 13.34 & 0.70 & 1.70 & 2.82 & & 0.97 & Gaia DR3 \\
173 & 07:43:49.53 & -15:14:24.1 & 13.88 & 0.64 & 42.68 & 9.27 & & 0.97 & Gaia DR3 \\
174 & 07:43:50.00 & -15:05:06.5 & 14.38 & 0.76 & 9.27 & 9.93 & & 1.03 & Gaia DR3 \\
175 & 07:43:56.02 & -15:07:14.3 & 9.35 & 0.62 & 49.16 & 0.37 & & 0.93 & Gaia DR3 \\
\hline
\end{tabular}
\label{tab:NGC_2437}
\end{table*}
